# Supplementary material for: NeuMan: Neural Human Radiance Field from a Single Video
Source: arXiv:2203.12575 source file (2022-09-22)
Supplement: Supplementary file 2 [file components_ablation.tex]

\begin{figure}[h]
\centering
\includegraphics[width=0.9\linewidth]{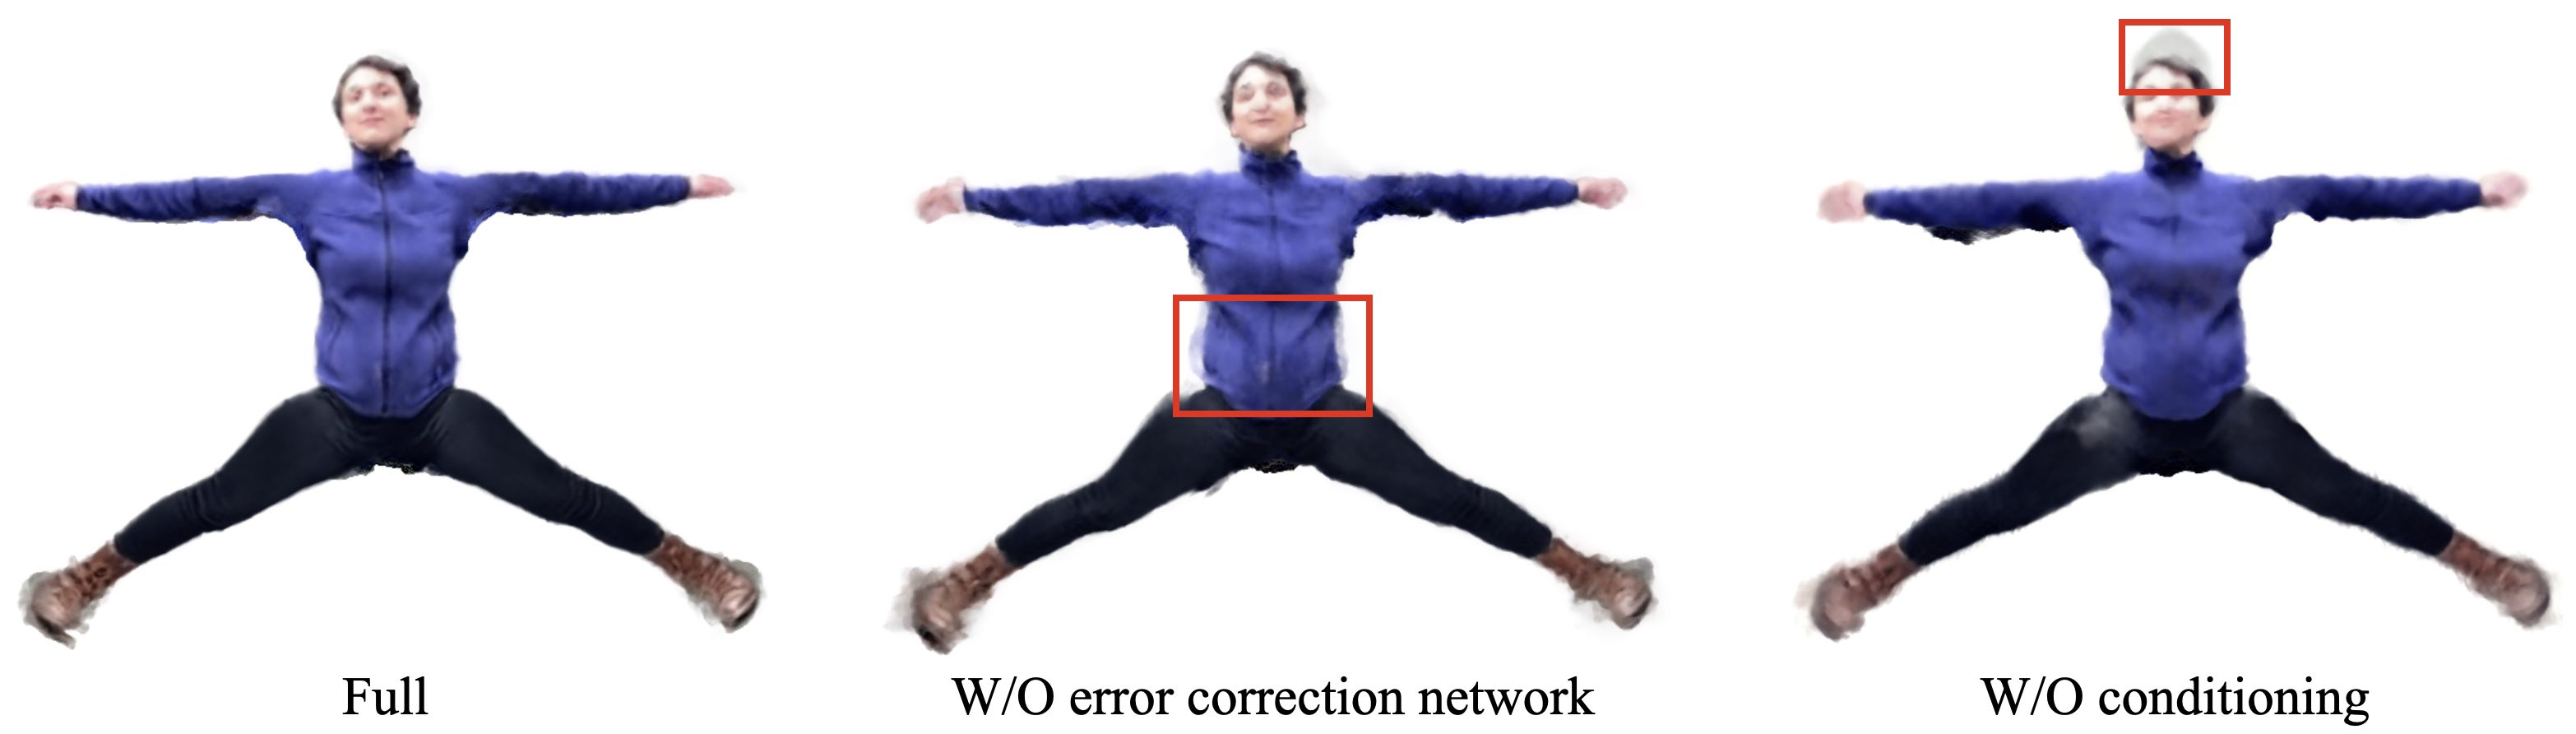}
\vspace{-1em}
\caption{
 Canonical renderings of our full model, model without error correction network, and model without conditioning on scene NeRF.
}
\vspace{-1.5em}
\label{fig:models_comp}
\end{figure}
\endinput
